# Supplementary material for: A Critical Re-evaluation of Benchmark Datasets for (Deep) Learning-Based Matching Algorithms
Source: arXiv:2307.01231 source file (2023-11-13)
Supplement: Supplementary file 1 [file appendix.tex]

Despite the same origin, our new benchmarks differ from the existing ones in the second step of our methodology. The benchmarks in Table \ref{tb:commonDatasets} were originally presented in~\cite{Mudgal2018sigmod}, where the authors state that blocking was applied with Magellan~\cite{DBLP:journals/pvldb/KondaDCDABLPZNP16}, without clarifying the exact method and corresponding parameter configuration that was used. As a result, the average imbalance ratio in these datasets is 16.4\% (see IR column in Table~\ref{tb:commonDatasets}), which means that the training, validation, and testing sets include around six negative instances per positive one. This is much lower in practice, as explained below.

More specifically, we apply DeepBlocker~\cite{DBLP:journals/pvldb/Thirumuruganathan21}
to the datasets in Table \ref{tb:newDatasets}. We configure DeepBlocker so that its recall, also known as pair completeness ($PC$)~\cite{Christen2012springer}, exceeds 90\%.
Such a high recall ensures realistic settings, given that $PC$ sets the upper bound of matching recall: the learning-based matchers we consider take decisions at the level of individual record pairs and, thus, they cannot infer more duplicates than those included in the candidate pairs.
